# Supplementary material for: Synchronizing Chaos with Imperfections
Source: arXiv:2104.13376 ancillary file (2021-04-27)
Supplement: Supplementary file 1 [file Supplemental_Material.pdf]

# SUPPLEMENTAL MATERIAL
# Synchronizing Chaos with Imperfections

Yoshiki Sugitani, Yuanzhao Zhang, and Adilson E. Motter

## S1. EXPERIMENTAL SETUP

Figure S1 shows an image of the circuits used in our experiments. Figure S1(a) presents the setup for five circuit oscillators connected through the coupling circuit. The coupling circuit controls the network structure and coupling strength, and it has LEDs attached to it to monitor the oscillations of the voltages $v_x^{(i)}$. An analog-to-digital converter (ADC: USB6210, National Instruments, sampling rate 25 kHz) is also attached to the coupling circuit to record the voltage data $v_x^{(i)}$ in a computer. The supply voltage to the op-amps (TL084) is ±9 V. The maximum tolerance of the resistors is 1% and that of the capacitors is 5% (except for the smallest capacitors, which is 10%). The op-amps have a maximum offset of 15 mV.

Figure S1(b) shows the circuit for a single oscillator. The tunable capacitor $C_y^{(i)}$ is implemented as an array consisting of one large capacitor and several small capacitors. We adjust the time scale $\tau_i$ by moving the small capacitors from one oscillator to another. This procedure allows us to change $\tau_i$ while keeping the average $\bar{C}_y$ constant. In Figs. 2 and 3, the capacitors $C_y^{(i)}$ are implemented starting with one large capacitor of 4.7 $\mu$F and 10 small capacitors of 0.1 $\mu$F for each oscillator. To satisfy the relations $C_y^{(i)} = 10C_x^{(i)}$ and $C_z^{(i)} = C_x^{(i)}$ in Eq. (4), the capacitors $C_x^{(i)}$ and $C_z^{(i)}$ are also implemented as modular capacitor arrays.

A similar procedure is used to adjust the heterogeneity in $\gamma_i$ by tuning $C_z^{(i)}$. In Fig. S6, we implement $C_z^{(i)}$ starting with an array composed of one large capacitor of 0.33 $\mu$F and 20 small capacitors of 0.01 $\mu$F for each oscillator, so that $C_z^{(i)}$ can be adjusted by moving small capacitors across oscillators. The other capacitors are fixed at $C_y^{(i)} = 5.3\,\mu$F and $C_x^{(i)} = 0.53\,\mu$F.

Finally, the coupling strength $k$ is controlled by the resistors $r$, which are identical for all coupling in the network (see Fig. 1). Given the values of $\eta$ and $R$ used in the experiment, the coupling strength values of $k = 5$ and 8.18 are realized by setting $r = 3.6\,\mathrm{k}\Omega$ and $r = 2.2\,\mathrm{k}\Omega$, respectively.

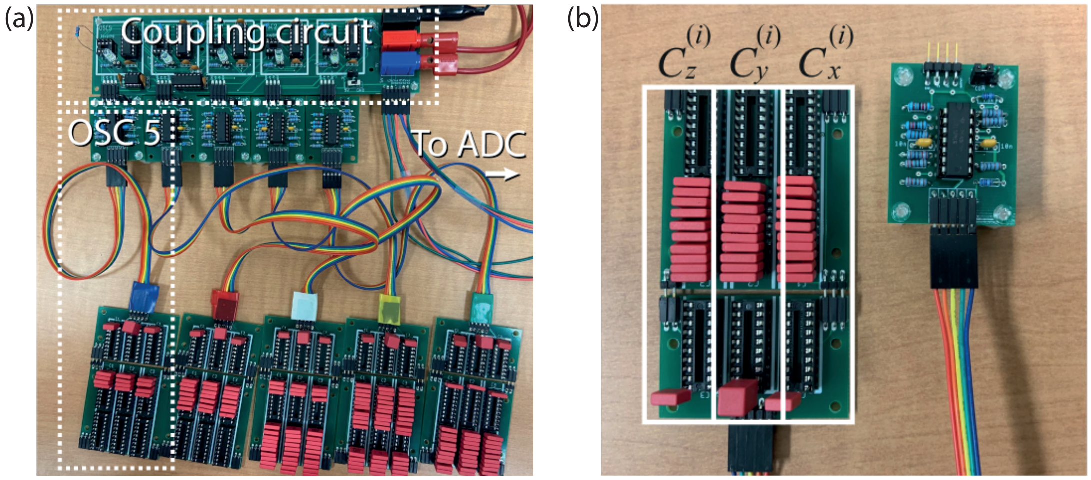


FIG. S1. Circuits used in the experiments. (a) Setup of the full circuit network. (b) Single-oscillator circuit, in which the time scale can be adjusted by varying the number of small capacitors.

## S2. SUPPLEMENTARY VIDEOS

Visualizations of the oscillator dynamics in Fig. 2(b) are available as Supplementary Videos. In these videos, the time series of the individual $v_x^{(i)}$ are captured by the light intensity of the LEDs, as illustrated by the snapshots in Fig. S2. The videos were recorded at 960 frames per second and are slowed down by a factor of 32 to facilitate visualization.

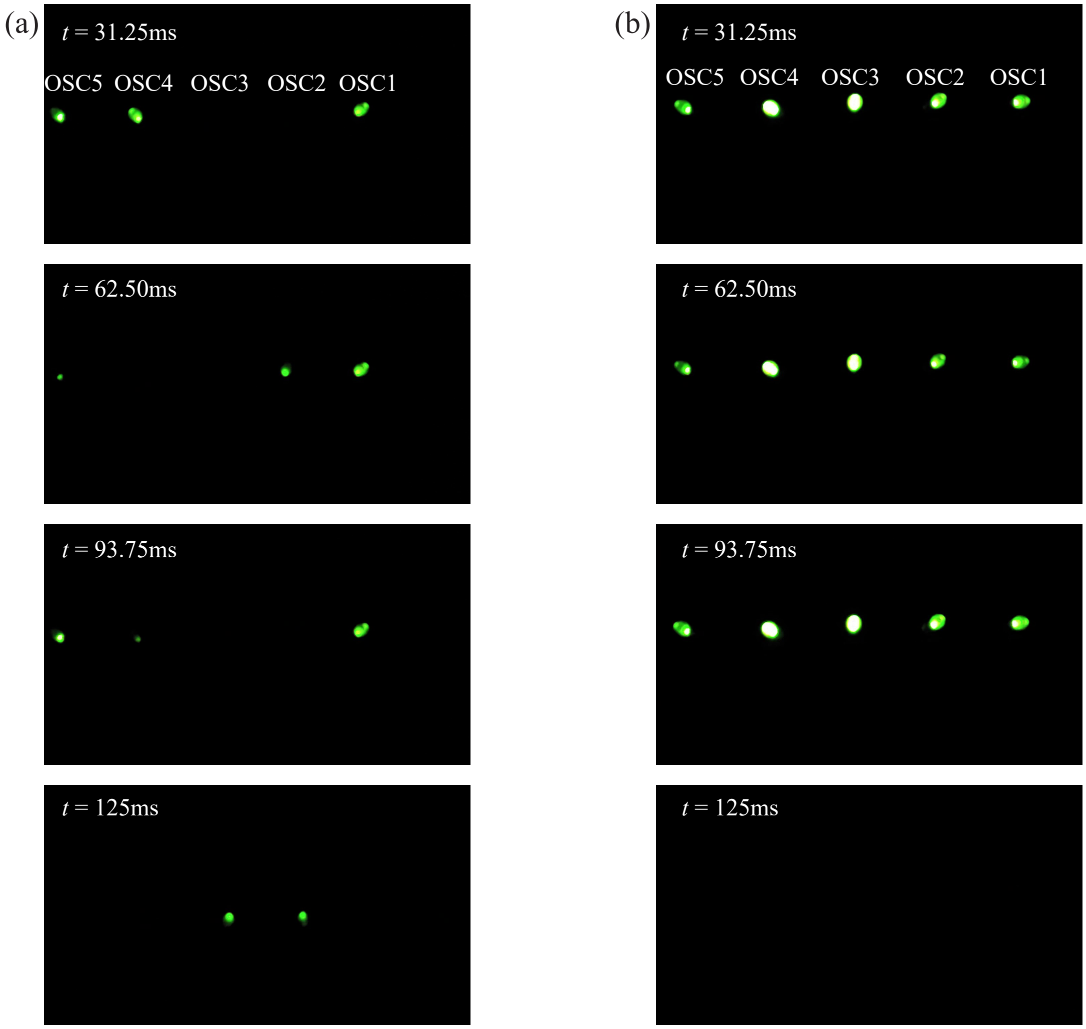


FIG. S2. Snapshots of the LEDs of the five oscillators in the directional ring network experiment of Fig. 2(b). (a) Oscillators with homogeneous time scales. (b) Oscillators with heterogeneous time scales. The images were recorded after the initial transient and show a clear contrast between the asynchronous dynamics of identical oscillators (a) and the synchronous dynamics of nonidentical ones (b).

## S3. NUMERICAL SIMULATIONS CAPTURE THE SYNCHRONIZING EFFECT OF OSCILLATOR HETEROGENEITY

To further substantiate our experimental findings, we perform numerical simulations using the model described by Eqs. (1)-(3). In order to mimic the voltage limit in the experiments, we impose the boundary conditions $\dot{x} = 0$ at $|x| = 7$ and $\dot{y} = 0$ at $|y| = 3$ in our model. Compared with the experiments, our numerical simulations show qualitatively similar transitions to synchronization in all directions of the parameter space $(\tau_1,\ \tau_2)$ as the heterogeneity is increased but for a slightly larger value of $\sigma$ (Fig. S3). This can be potentially explained by the intrinsic heterogeneities in the experiments, which further stabilize synchronization in the circuits. Given the idealized nature of our model (Chua's equations), the agreement between the experiments and simulations is impressive, and it indicates that the model successfully captures the essence of the experimental system.

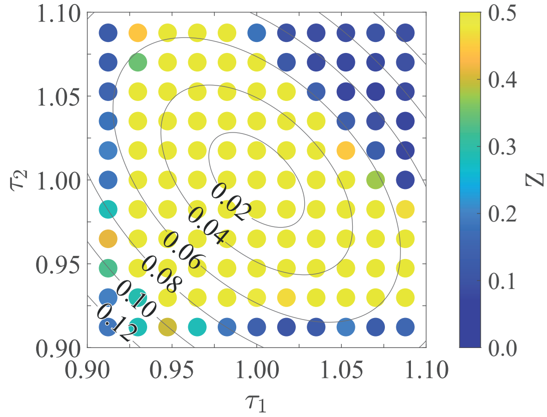


FIG. S3. Analog of Fig. 3 obtained from numerical simulations of Chua's equations. The synchronization error $Z$ at each point is determined from 36 simulation trials.

Figure S4 shows an expansion of Fig. S3 for a wider parameter range. The upper-right gray area represents the unphysical parameter region where $\tau_3 < 0$. The center of Fig. S4 corresponds to the homogeneous system with $\tau_i = 1.0$ for all $i$, and it is characterized by a large synchronization error $Z$. As we move away from the center, regardless of the direction, $Z$ decreases to a value close to zero. Further away from the center, $Z$ increases again and the oscillators lose synchrony, as expected from common intuition.

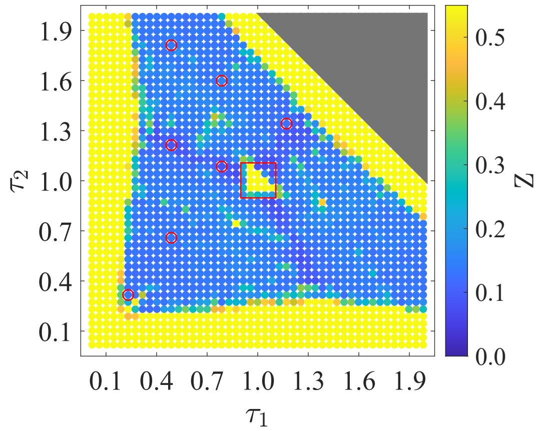


FIG. S4. Expansion of Fig. S3 showing the synchronization error $Z$ for a wide range of heterogeneous $\tau_i$. The red box corresponds to the original parameter range shown in Fig. S3. Typical time series for parameters marked by red circles are shown in Fig. S5.

To further understand Fig. S4, we show in Fig. S5 the time series for seven representative parameter sets for which the system synchronizes and compare them to the trajectory of an uncoupled oscillator with $\tau = 1$. We can see that the oscillators with smaller $\tau$ become entrained by the oscillator with the largest $\tau$ and, as a consequence, a common dynamical time scale emerges for the heterogeneous oscillators.

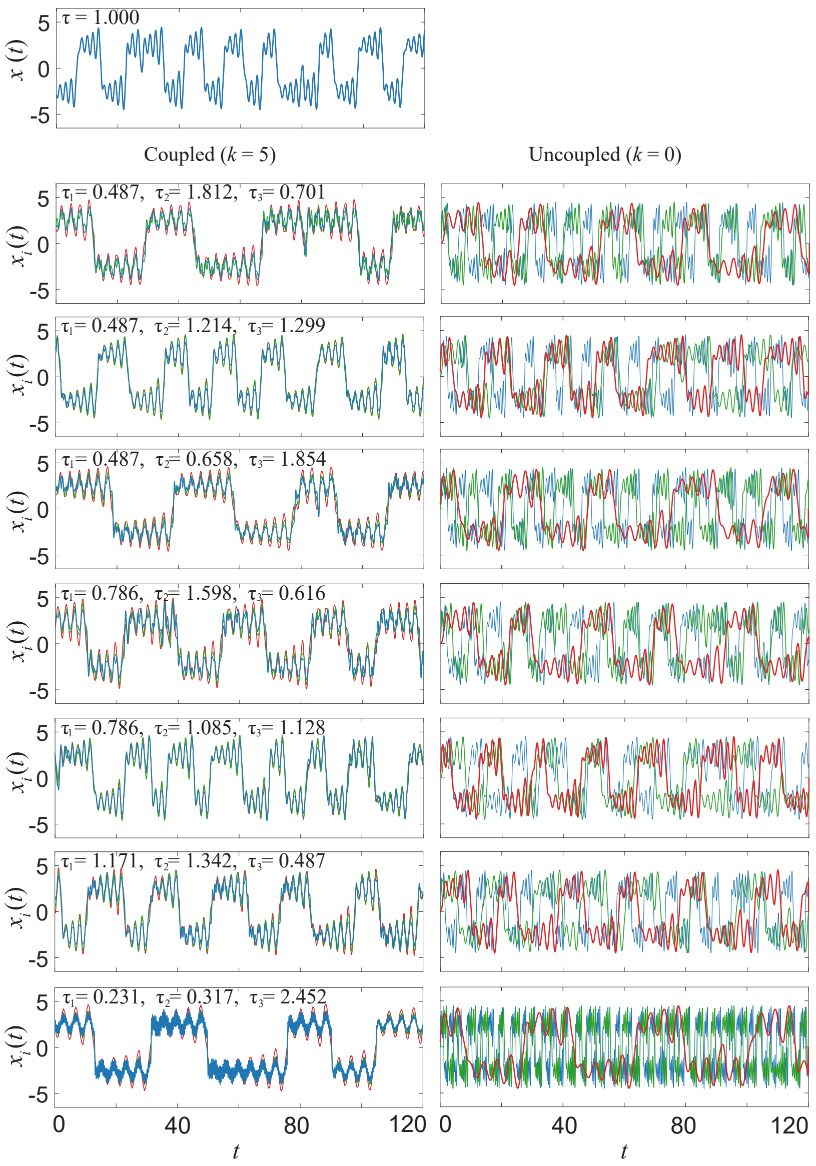


FIG. S5. Representative time series for seven different sets of heterogeneous time scales. For the uncoupled cases, the trajectory of the oscillator with the largest time scale $\tau$ is highlighted in red (with green and blue used respectively for the intermediate and the smallest $\tau$). For each parameter set, despite having very different time scales, the coupled oscillators synchronize to a common dynamical time scale. The time scale of the synchronous trajectory is strongly correlated with the time scale of the oscillator with the largest $\tau$ (compare left to the red trajectory on the right). The top panel shows the trajectory for an uncoupled oscillator with time scale $\tau = 1$ as a reference (which is also the trajectory of the unstable synchronization state of the network for the corresponding homogeneous time scales).

## S4. CHUA'S CIRCUITS WITH HETEROGENEITY IN OTHER PARAMETERS

In the paper we focused on the effect of heterogeneity in the time scales $\tau_i$. While the time scale is a natural parameter to consider, as it allows probing the effect of heterogeneity when the chaotic properties of the dynamics are manifestly preserved, the phenomenon reported here is not limited to $\tau_i$ and can also be observed for other parameters. This is illustrated in Fig. S6, where we relax the second condition in Eq. (4) to allow the parameter $\gamma$ to take different values $\gamma_i$ across different oscillators. The network and parameters are the same as in Fig. 3, except that in this case all $\tau_i$ are set to 1.0 and $\gamma_i$ are individually varied under the constraint that the average among the oscillators is kept fixed at $\bar{\gamma} = 0.056$. This is achieved experimentally by adjusting the capacitance $C_z^{(i)}$ for each oscillator $i$. We can see that the experimental data for $\gamma_i$ [Fig. S6(a)] show the same synchronization transition as observed for heterogeneous time scales $\tau_i$. The numerical results in Fig. S6(b) agree well with the experiments. Furthermore, our theoretical predictions of stability based on the largest Lyapunov exponents calculated from Eq. (10) [Fig. S6(c)] confirms the same synchronization transition at $\sigma \approx 0.007$.

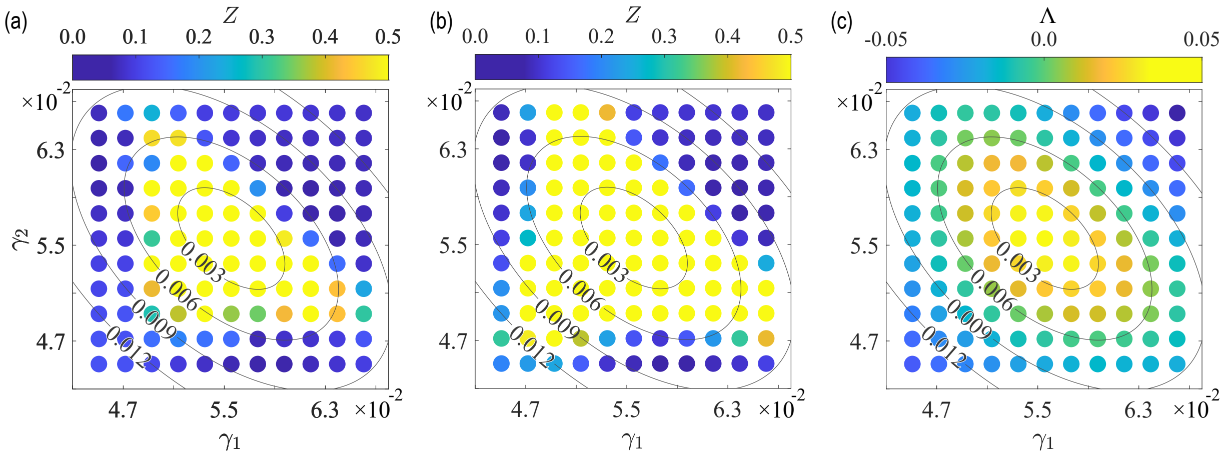


FIG. S6. Synchronizing effect of heterogeneity in $\gamma_i$ from (a) experiments, (b) numerical simulations, and (c) theoretical predictions. In each panel, the network and undeclared parameters are the same as in Fig. 3.

## S5. EXPERIMENTS ON CHUA'S CIRCUITS EXHIBITING SINGLE-SCROLL CHAOS

Figure S7 shows the experimental results for Chua's circuits exhibiting single-scroll chaos. To observe single-scroll chaos, we set $\gamma = 0.0455$ in Eq. (2), and the other parameters are the same as those in the paper. We implement this chaotic circuit experimentally by setting $R_2 = 2.2\,\mathrm{k}\Omega$ and $R_3 = 1.8\,\mathrm{k}\Omega$, while keeping the other parameters unchanged.

In Figs. S7(b) and (c), the coupling strength is below the synchronization threshold for the identical oscillators, and the homogeneous systems exhibit large synchronization error. In comparison, the heterogeneous systems show significantly smaller synchronization error and closely resemble the dynamics of a single oscillator.

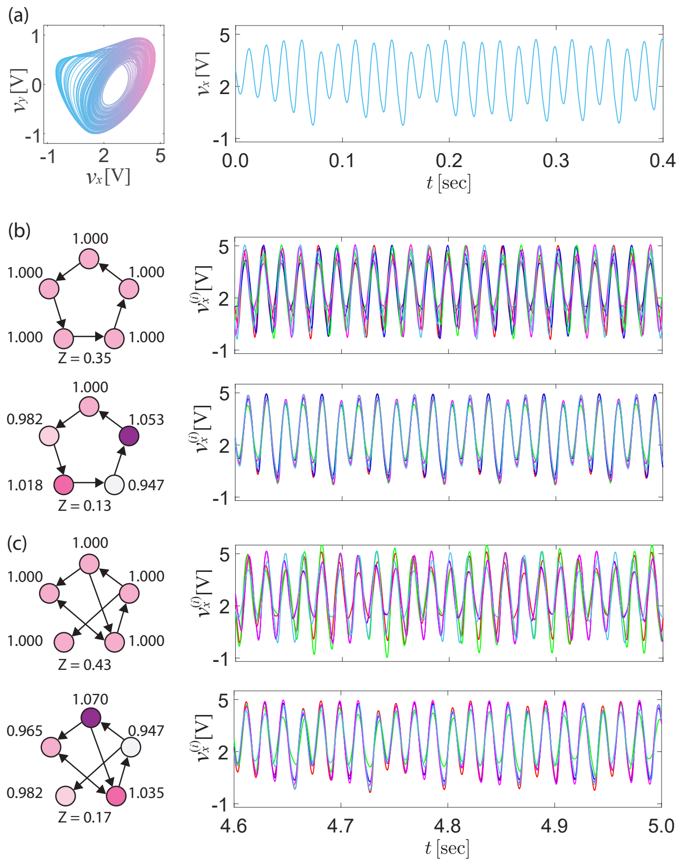


FIG. S7. Experimental time series of the voltage $v_x^{(i)}$ for single-scroll chaotic circuits. (a) Single-scroll chaotic attractor of an uncoupled oscillator and the corresponding time series. (b) Dynamics on a directed network for homogeneous and heterogeneous oscillators, respectively. (c) Dynamics on a random network for homogeneous and heterogeneous oscillators, respectively. The coupling strength is set to $k = 9.47$ in (b) and $k = 5.45$ in (c).

## S6. EXTENDED MASTER STABILITY FUNCTION

In this section, we prove that the Lyapunov exponents of each perturbation mode do not depend on oscillator heterogeneity according to the extended master stability function (MSF) originally developed in Ref. [25]. Consider a network of heterogeneous oscillators

$$\dot{\boldsymbol{x}}_i = \boldsymbol{F}(\boldsymbol{x}_i, p_i) - k \sum_{j=1}^{N} L_{ij} \boldsymbol{H}(\boldsymbol{x}_j, p_i), \tag{S1}$$

where $p_i$ is the parameter for the $i$th oscillator that is allowed to be heterogeneous.

Assuming that the parameter mismatches $\delta_i = p_i - \bar{p}$ are small, an extended MSF $\Lambda(\alpha,\beta)$ can be derived. By assuming that the original perturbation modes for the identical oscillators remain independent from each other, the extended MSF preserves the dimension reduction achieved in the original MSF formalism and can offer insights into many aspects of the synchronization dynamics of the heterogeneous oscillators (e.g., starting from a stable homogeneous system, it predicts that the synchronization error grows linearly with oscillator heterogeneity [25]). The function $\Lambda(\alpha,\beta)$ is the largest Lyapunov exponent of the variational equation

$$\dot{\boldsymbol{\xi}} = [\mathrm{D}_{\boldsymbol{x}} \boldsymbol{F}(\bar{\boldsymbol{x}}, \bar{p}) - \alpha \mathrm{D}_{\boldsymbol{x}} \boldsymbol{H}(\bar{\boldsymbol{x}}, \bar{p})] \boldsymbol{\xi} + \left[\mathrm{D}_p \boldsymbol{F}(\bar{\boldsymbol{x}}, \bar{p}) - \alpha \mathrm{D}_p \boldsymbol{H}(\bar{\boldsymbol{x}}, \bar{p})\right] \beta, \tag{S2}$$

where D represents the Jacobian operator and $\bar{\boldsymbol{x}}$ is the trajectory of a single oscillator with the parameter $p$ set to the mean value $\bar{p}$. Here, $\boldsymbol{\xi}$ is the perturbation mode that corresponds to the eigenvalue $\lambda$ of the modified graph Laplacian $\boldsymbol{G} = (G_{ij})$ defined by $G_{ij} = L_{ij} - \frac{1}{N} \sum_{i=1}^{N} L_{ij}$. The parameter $\alpha = k\lambda$ is determined by the coupling strength $k$ and the eigenvalue $\lambda$, and $\beta = \boldsymbol{w}^\intercal \boldsymbol{\delta}$ is the inner product of the parameter mismatch vector $\boldsymbol{\delta} = [\boldsymbol{\delta}_1^\intercal, \cdots, \boldsymbol{\delta}_N^\intercal]^\intercal$ and the left eigenvector $\boldsymbol{w}$ of $\boldsymbol{G}$ corresponding to $\lambda$.

Next, we show that the extended MSF $\Lambda(\alpha,\beta)$ does not depend on $\beta$, which encodes information about oscillator heterogeneity. This is most clearly demonstrated when we multiply both sides of Eq. (S2) by an arbitrary constant $c \neq 0$ and set $\boldsymbol{\eta} = c\boldsymbol{\xi}$:

$$\dot{\boldsymbol{\eta}} = [\mathrm{D}_{\boldsymbol{x}} \boldsymbol{F}(\bar{\boldsymbol{x}}, \bar{p}) - \alpha \mathrm{D}_{\boldsymbol{x}} \boldsymbol{H}(\bar{\boldsymbol{x}}, \bar{p})] \boldsymbol{\eta} + \left[\mathrm{D}_p \boldsymbol{F}(\bar{\boldsymbol{x}}, \bar{p}) - \alpha \mathrm{D}_p \boldsymbol{H}(\bar{\boldsymbol{x}}, \bar{p})\right] c\beta. \tag{S3}$$

Since the equation is unchanged from multiplying $c$ on both sides and $\boldsymbol{\eta}$ clearly has the same Lyapunov exponents as $\boldsymbol{\xi}$, we conclude that $\Lambda(\alpha,\beta) = \Lambda(\alpha, c\beta)$ for any $c \neq 0$. Using the fact that $\Lambda(\alpha,\beta)$ is a continuous function of $\beta$, we see that $\Lambda(\alpha,\beta)$ is constant for all $\beta \in \mathbb{C}$. Thus, according to the extended MSF, oscillator heterogeneity does not change the Lyapunov exponents (and the stability) of each perturbation mode.

## S7. MAPPING HETEROGENEOUS TIME SCALES TO THE MIXING AMONG PERTURBATION MODES

In the case of three unidirectionally coupled oscillators with heterogeneous $\tau_i$, Eq. (7) reads

$$\begin{aligned}
\delta\dot{\boldsymbol{X}} &= \left[\begin{pmatrix} 1/\tau_1 & 0 & 0 \\ 0 & 1/\tau_2 & 0 \\ 0 & 0 & 1/\tau_3 \end{pmatrix} \otimes \mathrm{D}\boldsymbol{F}(\boldsymbol{x}) - k \begin{pmatrix} 1/\tau_1 & 0 & -1/\tau_1 \\ -1/\tau_2 & 1/\tau_2 & 0 \\ 0 & -1/\tau_3 & 1/\tau_3 \end{pmatrix} \otimes \mathrm{D}\boldsymbol{H}(\boldsymbol{x})\right] \delta\boldsymbol{X}, \\
&= \left[\boldsymbol{I}_N \otimes \mathrm{D}\boldsymbol{F}(\boldsymbol{x}) - k\boldsymbol{L} \otimes \mathrm{D}\boldsymbol{H}(\boldsymbol{x}) + \left\{\begin{pmatrix} \hat{\tau}_1 & 0 & 0 \\ 0 & \hat{\tau}_2 & 0 \\ 0 & 0 & \hat{\tau}_3 \end{pmatrix} \otimes \mathrm{D}\boldsymbol{F}(\boldsymbol{x}) - k \begin{pmatrix} \hat{\tau}_1 & 0 & -\hat{\tau}_1 \\ -\hat{\tau}_2 & \hat{\tau}_2 & 0 \\ 0 & -\hat{\tau}_3 & \hat{\tau}_3 \end{pmatrix} \otimes \mathrm{D}\boldsymbol{H}(\boldsymbol{x})\right\}\right] \delta\boldsymbol{X},
\end{aligned} \tag{S4}$$

where $\hat{\tau}_i = 1/\tau_i - 1$.

By applying the transformation matrix $\boldsymbol{Q}$ that diagonalizes $\boldsymbol{L} = \left(\begin{smallmatrix} 1 & 0 & -1 \\ -1 & 1 & 0 \\ 0 & -1 & 1 \end{smallmatrix}\right)$,

$$\boldsymbol{Q} = \begin{pmatrix} 1 & \frac{1}{2}\left(-1 - \mathrm{i}\sqrt{3}\right) & \frac{1}{2}\left(-1 + \mathrm{i}\sqrt{3}\right) \\ 1 & \frac{1}{2}\left(-1 + \mathrm{i}\sqrt{3}\right) & \frac{1}{2}\left(-1 - \mathrm{i}\sqrt{3}\right) \\ 1 & 1 & 1 \end{pmatrix}, \tag{S5}$$

Eq. (S4) becomes

$$\dot{\boldsymbol{\xi}} = \left[\boldsymbol{I}_N \otimes \mathrm{D}\boldsymbol{F}(\boldsymbol{x}) - k\boldsymbol{\lambda} \otimes \mathrm{D}\boldsymbol{H}(\boldsymbol{x}) + \widetilde{\boldsymbol{\Delta}}(\boldsymbol{x})\right]\boldsymbol{\xi}, \tag{S6}$$

where

$$\begin{aligned}
\widetilde{\boldsymbol{\Delta}} = &\begin{pmatrix} \frac{1}{3}(\hat{\tau}_1 + \hat{\tau}_2 + \hat{\tau}_3) & \frac{1}{6}\left(\left(-1 - \mathrm{i}\sqrt{3}\right)\hat{\tau}_1 + \mathrm{i}\left(\sqrt{3} + \mathrm{i}\right)\hat{\tau}_2 + 2\hat{\tau}_3\right) & \frac{1}{6}\left(\mathrm{i}\left(\sqrt{3} + \mathrm{i}\right)\hat{\tau}_1 + \left(-1 - \mathrm{i}\sqrt{3}\right)\hat{\tau}_2 + 2\hat{\tau}_3\right) \\ \frac{1}{6}\left(\mathrm{i}\left(\sqrt{3} + \mathrm{i}\right)\hat{\tau}_1 + \left(-1 - \mathrm{i}\sqrt{3}\right)\hat{\tau}_2 + 2\hat{\tau}_3\right) & \frac{1}{3}(\hat{\tau}_1 + \hat{\tau}_2 + \hat{\tau}_3) & \frac{1}{6}\left(\left(-1 - \mathrm{i}\sqrt{3}\right)\hat{\tau}_1 + \mathrm{i}\left(\sqrt{3} + \mathrm{i}\right)\hat{\tau}_2 + 2\hat{\tau}_3\right) \\ \frac{1}{6}\left(\left(-1 - \mathrm{i}\sqrt{3}\right)\hat{\tau}_1 + \mathrm{i}\left(\sqrt{3} + \mathrm{i}\right)\hat{\tau}_2 + 2\hat{\tau}_3\right) & \frac{1}{6}\left(\mathrm{i}\left(\sqrt{3} + \mathrm{i}\right)\hat{\tau}_1 + \left(-1 - \mathrm{i}\sqrt{3}\right)\hat{\tau}_2 + 2\hat{\tau}_3\right) & \frac{1}{3}(\hat{\tau}_1 + \hat{\tau}_2 + \hat{\tau}_3) \end{pmatrix} \otimes \mathrm{D}\boldsymbol{F} \\
&-k \begin{pmatrix} 0 & \frac{1}{6}\left(\left(-3 - \mathrm{i}\sqrt{3}\right)\hat{\tau}_1 + 2\mathrm{i}\sqrt{3}\hat{\tau}_2 + \left(3 - \mathrm{i}\sqrt{3}\right)\hat{\tau}_3\right) & \frac{1}{6}\left(\mathrm{i}\left(\sqrt{3} + 3\mathrm{i}\right)\hat{\tau}_1 - 2\mathrm{i}\sqrt{3}\hat{\tau}_2 + \left(3 + \mathrm{i}\sqrt{3}\right)\hat{\tau}_3\right) \\ 0 & \frac{1}{6}\left(3 - \mathrm{i}\sqrt{3}\right)(\hat{\tau}_1 + \hat{\tau}_2 + \hat{\tau}_3) & \frac{1}{6}\left(-2\mathrm{i}\sqrt{3}\hat{\tau}_1 + \mathrm{i}\left(\sqrt{3} + 3\mathrm{i}\right)\hat{\tau}_2 + \left(3 + \mathrm{i}\sqrt{3}\right)\hat{\tau}_3\right) \\ 0 & \frac{1}{6}\left(2\mathrm{i}\sqrt{3}\hat{\tau}_1 + \left(-3 - \mathrm{i}\sqrt{3}\right)\hat{\tau}_2 + \left(3 - \mathrm{i}\sqrt{3}\right)\hat{\tau}_3\right) & \frac{1}{6}\left(3 + \mathrm{i}\sqrt{3}\right)(\hat{\tau}_1 + \hat{\tau}_2 + \hat{\tau}_3) \end{pmatrix} \otimes \mathrm{D}\boldsymbol{H}.
\end{aligned} \tag{S7}$$

Equation (S7) explicitly links the mixing between the perturbation modes to the values of $\tau_i$. The expression of $\widetilde{\boldsymbol{\Delta}}$ for heterogeneities in other oscillator parameters can be found similarly using the transformation matrix $\boldsymbol{Q}$.

## S8. IMPERFECTIONS SYNCHRONIZE CHAOS IN NON-AUTONOMOUS SYSTEMS

We consider the following forced nonlinear oscillators with damping:

$$\ddot{\theta}_i + \gamma\dot{\theta}_i = -\sin\theta_i + I + J\sin(\omega t + \phi_i) - k\sum_{j=1}^{N} L_{ij}\theta_j, \qquad i = 1, 2, \dots, N, \tag{S8}$$

which describes a wide range of systems from driven pendulums [17, 18] to Josephson junction [38, 39].

It has been shown previously that introducing heterogeneity can suppress chaos in systems described by Eq. (S8) [17], which sometimes lead to improved coherence with periodic collective dynamics [19]. Here, we show that heterogeneity in the parameter $\phi_i$ can induce synchronization without "killing" chaos, thus preserving the nature of the original dynamics. For this purpose, we set $\gamma = 0.75$, $I = 0.71466$, $J = 0.4$, and $\omega = 0.25$. Oscillators with these parameters evolve on the chaotic attractor shown in Fig. S8(a). When three such oscillators with identical $\phi_i$ are coupled unidirectionally at strength $k = 1.07$, they desynchronize due to transverse instability [Fig. S8(c)]. To restore synchrony, we introduce heterogeneity by setting $\phi_i$ to values drawn from a Gaussian distribution of standard deviation $\sigma = 0.02$. The three oscillators then remain synchronized close to the original chaotic attractor indefinitely [Figs. S8(b) and (d)]. This effect is robust to different realizations of the heterogeneity profile.

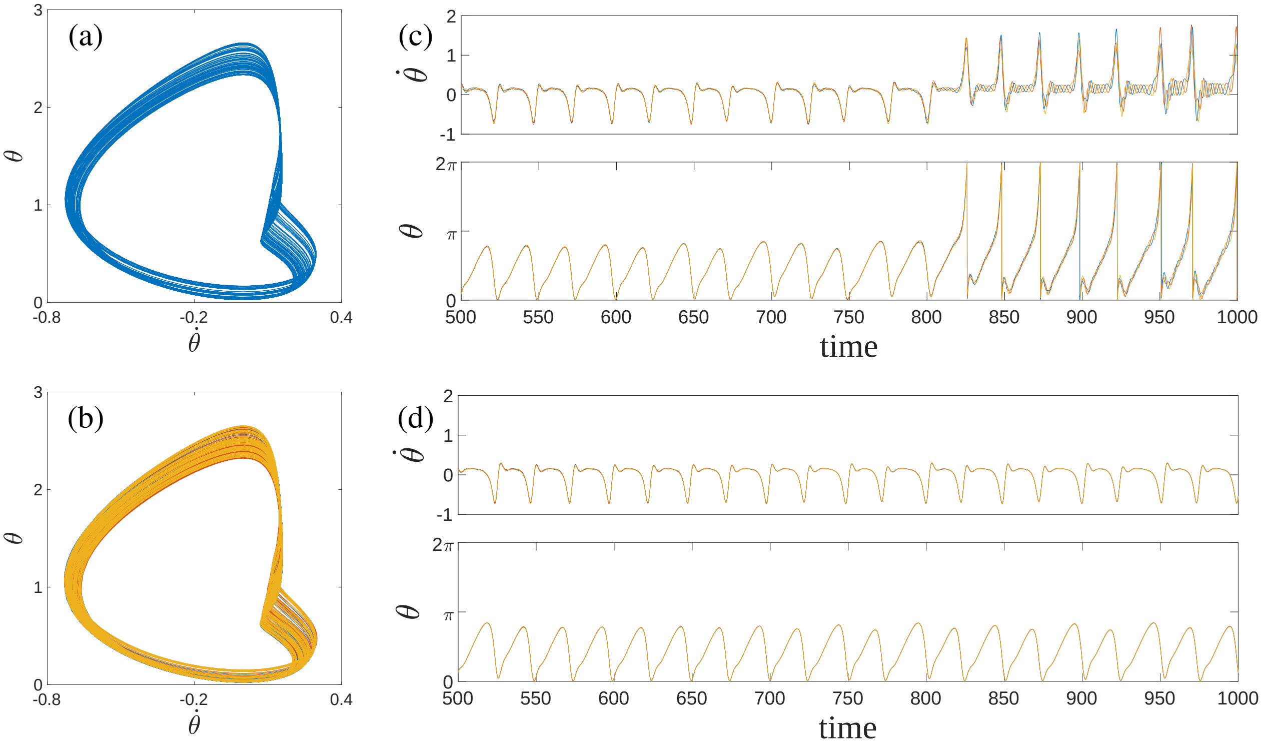


FIG. S8. Oscillator heterogeneity induces chaotic synchronization in a non-autonomous system. (a) Attractor of a single forced oscillator. The largest Lyapunov exponent of 0.016 indicates that the attractor is chaotic. (b) Attractor of three heterogeneous oscillators coupled unidirectionally with coupling strength $k = 1.07$. The heterogeneous parameter $\phi_i$ is drawn from a Gaussian distribution with $\sigma = 0.02$. The orbit of each oscillator is colored differently. (c) Typical trajectory of three identical oscillators coupled unidirectionally as in Fig. 3, with coupling strength $k = 1.07$. The oscillators desynchronize around $t = 800$. The normalized average synchronization errors for the steady state are $e_\theta = 0.03$ and $e_{\dot{\theta}} = 0.08$. (d) Typical trajectory of the three heterogeneous oscillators from (b). The oscillators remain synchronized around the original attractor of a single oscillator for all time $t$. The normalized average synchronization errors for the steady state are $e_\theta = 0.001$ and $e_{\dot{\theta}} = 0.003$.
